# Supplementary material for: Optical levitation of fluorescent silicon carbide nanoparticles in vacuum
Source: arXiv:2504.18653 source file (2025-04-25)
Supplement: Supplementary file 1 [file SiC_Optical_levitation_SM_np.pdf]

## Supplementary Material:

### Optical levitation of fluorescent silicon carbide nanoparticles in vacuum

Seyed Khalil Alavi,<sup>1,2</sup> Cheng-I Ho,<sup>3,2</sup> Iuliia Neumann,<sup>4</sup> Daniel Eberle,<sup>1,2</sup> Vadim Vorobyov,<sup>3,2</sup> Bertold Rasche,<sup>4</sup> and Sungkun Hong<sup>1,2</sup>

<sup>1)</sup>*Institute for Functional Matter and Quantum Technologies, University of Stuttgart, 70569, Stuttgart, Germany*

<sup>2)</sup>*Center for Integrated Quantum Science and Technology (IQST), University of Stuttgart, 70569, Stuttgart, Germany*

<sup>3)</sup>*3rd Institute of Physics, University of Stuttgart, 70569, Stuttgart, Germany*

<sup>4)</sup>*Institute of Inorganic Chemistry, University of Stuttgart, 70569, Stuttgart, Germany*

(\*Electronic mail: sungkun.hong@fmq.uni-stuttgart.de)

(\*Electronic mail: skalavi@fmq.uni-stuttgart.de)

(Dated: 25 April 2025)

## I. CONFOCAL CHARACTERIZATION OF THE SiC NANOPARTICLES

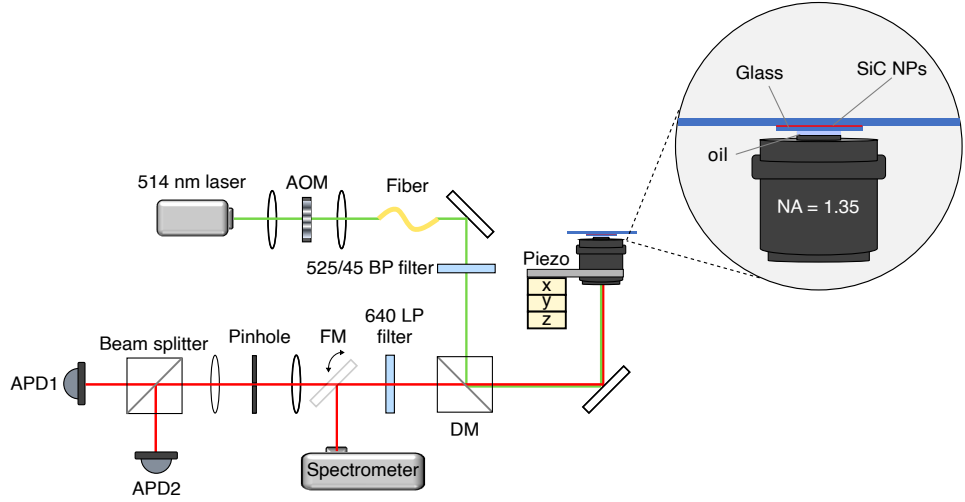

FIG. S1. Schematic of the scanning confocal microscope setup used to characterize the SiC nanoparticle (NP) sample. The 514 nm excitation laser is focused onto SiC nanoparticles (NP) on a glass substrate by a high-NA (NA = 1.35) oil immersion objective. An additional microscope slide is placed on the NP side to avoid direct contact with the immersion oil. The fluorescence photons emitted by the NP are collected by the same objective and guided to the detection setup. A dichroic mirror (DM) with a cut-off wavelength of 567 nm is used to separate the excitation laser path and the detection path. A 50/50 beam splitter distributes the fluorescence photons into two single-photon avalanche photodiode (APD) detectors. In order to obtain a confocal fluorescence map, the objective is scanned by a piezo stage and the fluorescence intensity is synchronously registered by summing the counts from the two APDs. The  $g^{(2)}(\tau)$  is measured by correlating the photon counts between two APDs. To obtain the emission spectra of the NP, a flip-mirror (FM) is flipped to direct the fluorescence to a spectrometer (Ocean QPro, wavelength range: 417.61 - 801.27 nm).

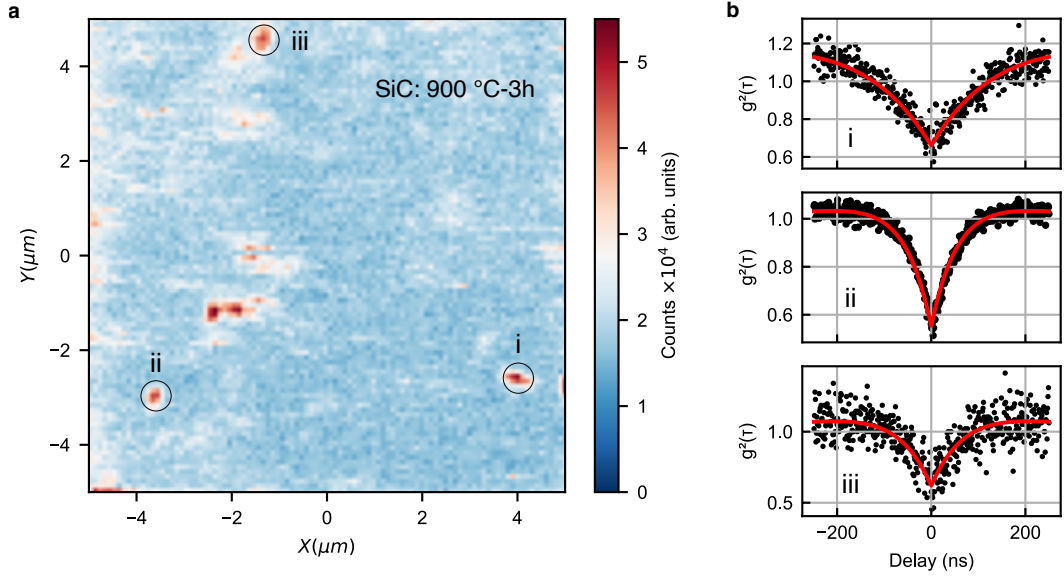

FIG. S2. **a** Confocal scanning microscope image of the similarly prepared SiC particles on glass. **b** Second-order intensity correlation  $g^{(2)}(\tau)$  of the fluorescence spot indicated in (a) by circles. All showed significant antibunching at  $\tau = 0$ , confirming characteristics of their single photon emission.

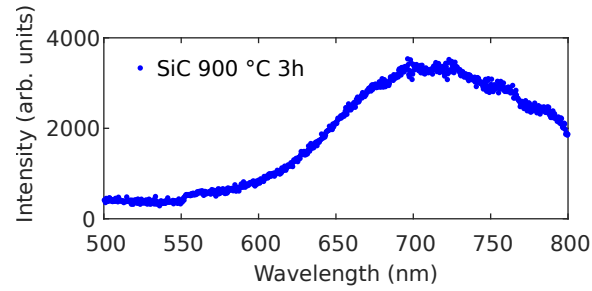

FIG. S3. Fluorescence emission spectrum of the SiC NP sample annealing at 900°C for 3 hours. It shows pronounced emission at a wavelength of about 700 nm, consistent with the observations reported in the previous study<sup>1</sup>.

## II. OXIDATION OF SiC NANOPARTICLES

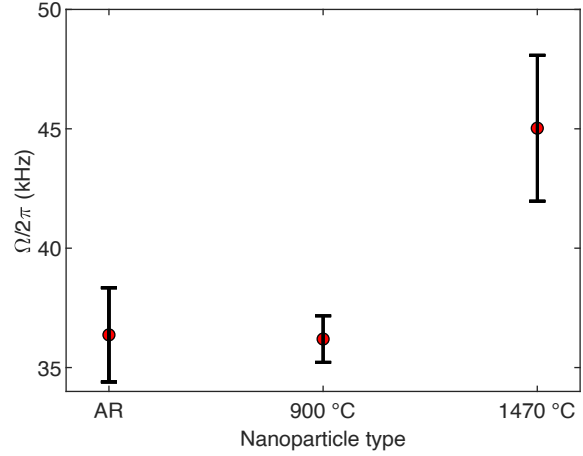

FIG. S4. Effects of annealing on the particle's frequency along the z-axis ( $\Omega_z/2\pi$ ) for samples prepared under different annealing conditions: SiC NP powders as received (AR), after annealing at 900°C for 24 hours (900°C), and after annealing at 1470°C for 24 hours (1470°C). The frequencies of the particle in the trap scale with the ratio of polarizability to density, which is different for SiC and SiO<sub>2</sub>. The results show a systematic increase in the particle's oscillation frequency with increased annealing severity, indicating compositional change of the SiC NP due to annealing.

To determine the exact composition of the nanoparticles after oxidation, the samples were heated in synthetic air (21 % O<sub>2</sub>, 79 % N<sub>2</sub>) from 30 °C to 1450 °C at a heating rate of 2 K/min employing thermo-gravimetry (TG), which records the mass change over temperature (Fig. S5). The thermal oxidation from SiC to SiO<sub>2</sub> begins at approximately 1000 °C, following the chemical equation:

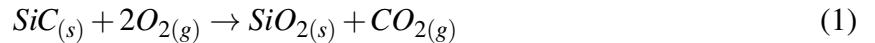

Due to the different molar masses of SiC and SiO<sub>2</sub> of 40.1 and 60.1 g/mol, respectively, we expect a gain in mass for this oxidation reaction. Comparing the actually observed gain in mass with the theoretically expected gain for a full oxidation, we can extract the percentage of SiC which remains unreacted:

$$\frac{m_f}{m_i} = \frac{m_f(\text{SiO}_2) + m_f(\text{SiC})}{m_i(\text{SiC})} = \frac{n_f(\text{SiO}_2) \times M(\text{SiO}_2) + n_f(\text{SiC}) \times M(\text{SiC})}{n_i(\text{SiC}) \times M(\text{SiC})}, \quad (2)$$

where  $m(\text{SiO}_2)$  ( $m(\text{SiC})$ ) is the mass of SiO<sub>2</sub> (SiC),  $n(\text{SiO}_2)$  ( $n(\text{SiC})$ ) is the number of moles of SiO<sub>2</sub> (SiC), and  $M(\text{SiO}_2)$  ( $M(\text{SiC})$ ) is the molar mass of SiO<sub>2</sub> (SiC). For a full oxidation

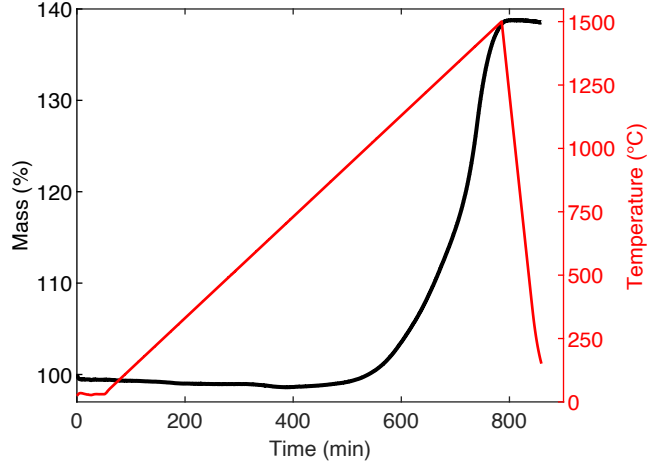

FIG. S5. Thermo-gravimetric measurement with the mass curve (black) for a sample of the SiC-NPs heated to 1450 °C at 2 K/min in synthetic air (21% O<sub>2</sub> and 79% N<sub>2</sub>) and subsequently cooled at 20 K/min to room temperature. Temperature is shown in red.

( $n_f(\text{SiO}_2) = n_i(\text{SiC})$  and  $n_f(\text{SiC}) = 0$ ; where  $f$  and  $i$  denote the final and initial, respectively) this becomes 1.5 or 150 %.

From the TG plot, we get a 140 % mass gain, which then translates into  $\frac{n_f(\text{SiC})}{n_f(\text{SiC}) + n_f(\text{SiO}_2)} = 20\%$ , meaning the NPs will consist of a core of 20 % SiC and a shell of 80 % SiO<sub>2</sub>. Considering an initial diameter of the NP of 90 nm (manufacturer data: 80 to 100 nm), we estimate the diameter of the remaining SiC core to be approximately 52.6 nm. We note that since oxygen diffusion at these high temperatures will be substantial, prolonged exposure (e.g., in our case for 24 h) will also likely further decrease the amount of SiC.

## REFERENCES

- <sup>1</sup>S. Castelletto, B. C. Johnson, C. Zachreson, D. Beke, I. Balogh, T. Ohshima, I. Aharonovich, and A. Gali, “Room temperature quantum emission from cubic silicon carbide nanoparticles,” *ACS Nano* **8**, 7938–7947 (2014).
